# Supplementary material for: Rethinking Trajectory Forecasting Evaluation
Source: arXiv:2107.10297 source file (2021-07-21)
Supplement: Supplementary file 1 [file appendix.tex]

\appendix

\section{Discrete-Time Unicycle Kinematics}
Take $\mathbf{s}^{(t)} = [x^{(t)}, y^{(t)}, \phi^{(t)}]^T$ and $\mathbf{u}^{(t)} = [u_v^{(t)}, u_\omega^{(t)}]^T$.

\begin{equation}\label{eqn:supp_unicycle_kin}
    \begin{bmatrix}
    x^{(t+1)} \\
    y^{(t+1)} \\
    \phi^{(t+1)}
    \end{bmatrix} = \begin{bmatrix}
    x^{(t)} \\
    y^{(t)} \\
    \phi^{(t)}
    \end{bmatrix} + \begin{bmatrix}
    u_v^{(t)} \cdot \cos(\phi^{(t)} + u_\omega^{(t)}) \Delta t\\
    u_v^{(t)} \cdot \sin(\phi^{(t)} + u_\omega^{(t)}) \Delta t\\
    u_\omega^{(t)}
    \end{bmatrix}.
\end{equation}
Thus:
\begin{equation}\label{eqn:supp_unicycle_kin_AB}
\begin{aligned}
    \mathbf{A}^{(t)} &= \frac{d \mathbf{f}}{d \mathbf{s}^{(t)}} = \begin{bmatrix}
    1 & 0 & - u_v^{(t)} \cdot \sin(\phi^{(t)} + u_\omega^{(t)}) \Delta t\\
    0 & 1 & u_v^{(t)} \cdot \cos(\phi^{(t)} + u_\omega^{(t)}) \Delta t\\
    0 & 0 & 1
    \end{bmatrix},\\
    \mathbf{B}^{(t)} &= \frac{d \mathbf{f}}{d \mathbf{u}^{(t)}} = \begin{bmatrix}
    \cos(\phi^{(t)} + u_\omega^{(t)}) \Delta t & - u_v^{(t)} \cdot \sin(\phi^{(t)} + u_\omega^{(t)}) \Delta t\\
    \sin(\phi^{(t)} + u_\omega^{(t)}) \Delta t & u_v^{(t)} \cdot \cos(\phi^{(t)} + u_\omega^{(t)}) \Delta t\\
    0 & 1
    \end{bmatrix}
\end{aligned}
\end{equation}

\section{Discrete-Time Unicycle Dynamics}
Take $\mathbf{s}^{(t)} = [x^{(t)}, y^{(t)}, \phi^{(t)}]^T$ and $\mathbf{u}^{(t)} = [u_v^{(t)}, u_\omega^{(t)}]^T$.

If $u_\omega^{(t)} = 0$:
\begin{equation}\label{eqn:supp_unicycle_dyn_zero_om}
    \begin{bmatrix}
    x^{(t+1)} \\
    y^{(t+1)} \\
    \phi^{(t+1)}
    \end{bmatrix} = \begin{bmatrix}
    x^{(t)} \\
    y^{(t)} \\
    \phi^{(t)}
    \end{bmatrix} + \begin{bmatrix}
    u_v^{(t)} \cdot \cos(\phi^{(t)}) \Delta t\\
    u_v^{(t)} \cdot \sin(\phi^{(t)}) \Delta t\\
    0
    \end{bmatrix}.
\end{equation}
If $u_\omega^{(t)} \neq 0$:
\begin{equation}\label{eqn:supp_unicycle_dyn}
\begin{aligned}
    \begin{bmatrix}
    x^{(t+1)} \\
    y^{(t+1)} \\
    \phi^{(t+1)}
    \end{bmatrix} &= \begin{bmatrix}
    x^{(t)} \\
    y^{(t)} \\
    \phi^{(t)}
    \end{bmatrix} + \begin{bmatrix}
    u_v^{(t)} \cdot D_S^{(t)}\\
    - u_v^{(t)} \cdot D_C^{(t)}\\
    u_\omega^{(t)} \Delta t
    \end{bmatrix},\\
    \text{where } D_S^{(t)} &= \frac{\sin(\phi^{(t)} + u_\omega^{(t)} \Delta t) - \sin(\phi^{(t)})}{u_\omega^{(t)}},\\
    D_C^{(t)} &= \frac{\cos(\phi^{(t)} + u_\omega^{(t)} \Delta t) - \cos(\phi^{(t)})}{u_\omega^{(t)}}.
\end{aligned}
\end{equation}
Thus, when $u_\omega^{(t)} = 0$:
\begin{equation}\label{eqn:supp_unicycle_AB_zero_om}
\begin{aligned}
    \mathbf{A}^{(t)} &= \frac{d \mathbf{f}}{d \mathbf{s}^{(t)}} = \begin{bmatrix}
    1 & 0 & -u_v^{(t)} \cdot \sin(\phi^{(t)}) \Delta t\\
    0 & 1 & u_v^{(t)} \cdot \cos(\phi^{(t)}) \Delta t\\
    0 & 0 & 1
    \end{bmatrix},\\
    \mathbf{B}^{(t)} &= \frac{d \mathbf{f}}{d \mathbf{u}^{(t)}} = \begin{bmatrix}
    \cos(\phi^{(t)}) \Delta t & 0\\
    \sin(\phi^{(t)}) \Delta t & 0\\
    0 & 0
    \end{bmatrix}.
\end{aligned}
\end{equation}
Finally, when $u_\omega^{(t)} \neq 0$:
\begin{equation}\label{eqn:supp_unicycle_AB}
\begin{aligned}
    \mathbf{A}^{(t)} &= \frac{d \mathbf{f}}{d \mathbf{s}^{(t)}} = \begin{bmatrix}
    1 & 0 & u_v^{(t)} \cdot D_C^{(t)}\\
    0 & 1 & u_v^{(t)} \cdot D_S^{(t)}\\
    0 & 0 & 1
    \end{bmatrix},\\
    \mathbf{B}^{(t)} &= \frac{d \mathbf{f}}{d \mathbf{u}^{(t)}} = \begin{bmatrix}
    D_S^{(t)} & B_{12}^{(t)}\\
    -D_C^{(t)} & B_{22}^{(t)}\\
    0 & \Delta t
    \end{bmatrix},\\
    \text{where } B_{12}^{(t)} &= \frac{u_v^{(t)}}{u_\omega^{(t)}} \cdot \left[ \cos(\phi^{(t)} + u_\omega^{(t)} \Delta t) \Delta t - D_S^{(t)} \right],\\
    B_{22}^{(t)} &= \frac{u_v^{(t)}}{u_\omega^{(t)}} \cdot \left[ \sin(\phi^{(t)} + u_\omega^{(t)} \Delta t) \Delta t + D_C^{(t)} \right].
\end{aligned}
\end{equation}
